# Supplementary material for: Bayesian Variable Selection for Function-on-Scalar Regression Models: a comparative analysis
Source: arXiv:2303.03521 ancillary file (2026-03-29)
Supplement: Supplementary file 1 [file supplementary_material.pdf]

# Bayesian Variable Selection for Function-on-Scalar Regression Models: a comparative analysis

## Supplementary Material

Pedro Henrique T. O. Sousa<sup>1\*</sup>, Camila P. E. de Souza<sup>2</sup>, Ronaldo Dias<sup>1</sup>

<sup>1</sup>Department of Statistics, Federal University of Paraná, Curitiba, PR, Brazil

<sup>2</sup>Department of Statistical and Actuarial Sciences, University of Western Ontario, ON, Canada

<sup>3</sup>Department of Statistics, University of Campinas, Campinas, SP, Brazil

\*Correspondence: pedro.henrique3@ufpr.br

### 1 Linear coefficient transformations

Regarding the estimates of the coefficients and functional intercept, it is important to recall that a standardization of the covariates was carried out in a phase prior to applying the proposed model. Thus, for all  $i$ , we have the following:

$$Z_l \beta_l(\cdot) X_{li} = Z_l \beta_l(\cdot) s_l \frac{(X_{li} - \bar{X}_l)}{s_l} + Z_l \beta_l(\cdot) \bar{X}_l,$$

in which  $\bar{X}_l$  and  $s_l$  represent the mean and standard deviation of the  $l$ th covariate, respectively. Therefore, after standardization, the  $l$ th partial functional coefficient is, in fact, the quantity  $s_l \beta_l(\cdot)$ , instead of only  $\beta_l(\cdot)$ . Note that the quantity  $Z_l \beta_l(\cdot) \bar{X}_l$  is not linked to  $X_{li}$  by multiplication and, therefore, is only aggregated to the intercept.

In other words, we have a linear transformation of the original partial functional coefficient. Thus, there is:

$$\tilde{\beta}_l(\cdot) = s_l \hat{\beta}_l(\cdot),$$

in which  $\tilde{\beta}_l(\cdot)$  is the estimate of the  $l$ th partial functional coefficient obtained by fitting the model when using standardized covariates, while  $\hat{\beta}_l(\cdot)$  is the estimate of the original  $l$ th partial functional coefficient, meaning the one returned by fitting the model without standardized covariates.

Bearing in mind the way in which the data were generated, the interest here is to know the value of  $\hat{\beta}_l(\cdot)$ , so that it is possible to compare it with  $\beta_l(\cdot)$  used in the generation of synthetic data. So, it is necessary to obtain  $\hat{\beta}_l(\cdot)$  from:

$$\hat{\beta}_l(\cdot) = \frac{1}{s_l} \tilde{\beta}_l(\cdot).$$

Similarly, the simple functional mean of the functional responses is an estimate for the intercept when using the standardized covariates, and this is also a linear transformation of what the intercept estimate would be if the covariates were considered without

standardization. Then, we have the following expression for the intercept:

$$\hat{\beta}_0(.) = \tilde{\beta}_0(.) - \sum_{l=1}^p \hat{Z}_l \left( \frac{1}{s_l} \tilde{\beta}_l(.) \right) \overline{X}_l, \quad (1)$$

in which  $\tilde{\beta}_0(.)$  is the simple functional mean of the functional responses, while  $\hat{\beta}_0(.)$  is the estimate of the true functional intercept ( $\beta_0(t) = \exp(t^2)$ , in the Manuscript Section 3.1). Therefore, in Expression 1, it is noticed that only the covariates that were selected by the model are contemplated.

Finally, it is worth mentioning that  $\hat{\beta}_0(.)$  is calculated according to the Expression (1) and carries the estimation errors of the simple functional mean and the coefficients  $\tilde{\beta}_l(.)$ 's. This accumulation of errors does not interfere with the final prediction values for the functional response, since

$$\hat{y}_i(.) = \hat{\beta}_0(.) + \sum_{l=1}^p \hat{Z}_l \hat{\beta}_l(.) X_{li} = \tilde{\beta}_0(.) + \sum_{l=1}^p \hat{Z}_l \tilde{\beta}_l(.) X S_{li}, \quad (2)$$

in which  $X S_{li}$  represents the  $l$ th covariate standardized by mean and standard deviation for the  $i$ th individual. Therefore, the quantities  $\hat{\beta}_0(.)$  and  $\hat{\beta}_l(.)$ 's are used in this paper only for graphical comparison with the actual parameters, while the quantities  $\tilde{\beta}_0(.)$  and  $\tilde{\beta}_l(.)$ 's can be used directly for the computation of functional predictions.

## 2 Supplementary tables

Table 1: MSEs of the proposed Bayesian approach with  $\mu$  as a hyperparameter and as a parameter, according to the different configurations of  $K$  B-spline basis functions, two dataset lengths ( $m \in \{10, 15\}$ ) and two noise variances,  $\sigma^2 = (0.2)^2$  and  $\sigma^2 = (20)^2$ .

| $\sigma$ | $m$ | $K$ | $\mu$ (Hyperparameter) |          |          |          |          |          |          |          |          | $\mu$ (Parameter) |
|----------|-----|-----|------------------------|----------|----------|----------|----------|----------|----------|----------|----------|-------------------|
|          |     |     | 0.1                    | 0.2      | 0.3      | 0.4      | 0.5      | 0.6      | 0.7      | 0.8      | 0.9      |                   |
| 0.2      | 5   | 5   | 0.90531                | 0.90336  | 0.88969  | 0.88341  | 0.91821  | 0.91849  | 0.89837  | 0.89995  | 0.91710  | 0.88802           |
|          | 10  | 10  | 0.08700                | 0.15229  | 0.19107  | 0.14702  | 0.13304  | 0.15841  | 0.10374  | 0.12840  | 0.09280  | 0.21730           |
|          |     | 15  | 0.46405                | 0.32608  | 0.39309  | 0.74008  | 0.45050  | 0.41925  | 0.43491  | 0.52743  | 0.55020  | 0.64612           |
|          | 5   | 5   | 0.91527                | 0.91841  | 0.91653  | 0.91829  | 0.91293  | 0.92054  | 0.92025  | 0.92007  | 0.91930  | 0.92293           |
|          | 15  | 10  | 0.02716                | 0.03917  | 0.02872  | 0.02942  | 0.01801  | 0.02089  | 0.02890  | 0.02723  | 0.01994  | 0.02456           |
|          |     | 15  | 0.09215                | 0.07390  | 0.16706  | 0.12765  | 0.10490  | 0.06630  | 0.16293  | 0.07826  | 0.05692  | 0.06983           |
| 20       | 5   | 5   | 36.26610               | 36.16406 | 34.79331 | 35.99577 | 32.02700 | 30.50700 | 33.82998 | 39.78591 | 38.77678 | 36.08834          |
|          | 10  | 10  | 48.26145               | 39.24513 | 43.34065 | 46.52245 | 44.98702 | 48.97598 | 54.27919 | 43.12962 | 48.73781 | 42.22430          |
|          |     | 15  | 75.35545               | 70.10816 | 66.12114 | 76.12941 | 85.12853 | 67.12481 | 64.62520 | 73.46087 | 60.47929 | 61.64159          |
|          | 5   | 5   | 18.34214               | 17.21293 | 17.09297 | 34.03930 | 32.26425 | 30.61627 | 28.33563 | 31.57612 | 36.45118 | 19.08434          |
|          | 15  | 10  | 28.82329               | 29.70966 | 34.56420 | 31.83856 | 32.22336 | 29.52405 | 31.30894 | 31.57785 | 46.33399 | 28.78035          |
|          |     | 15  | 45.94990               | 45.65931 | 43.40093 | 49.07942 | 45.36731 | 40.10978 | 47.95165 | 45.63433 | 45.05256 | 45.74638          |

### 3 Supplementary figures

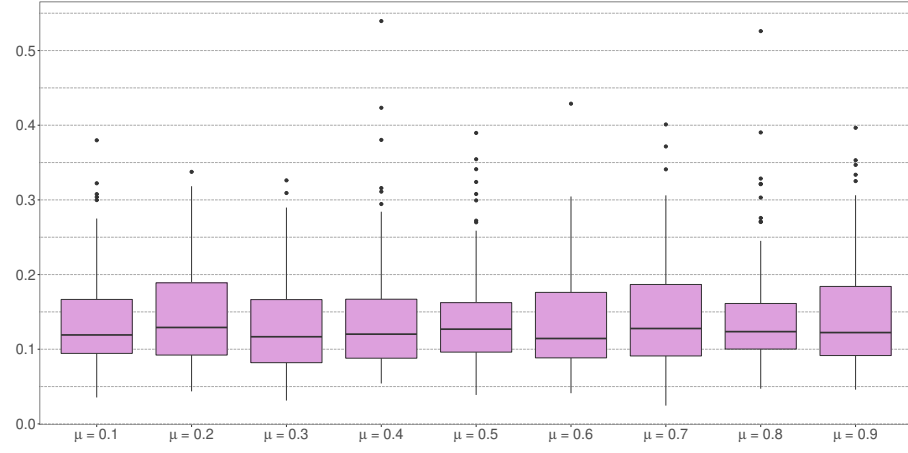

(a) Data with  $\sigma = 0.2$ .

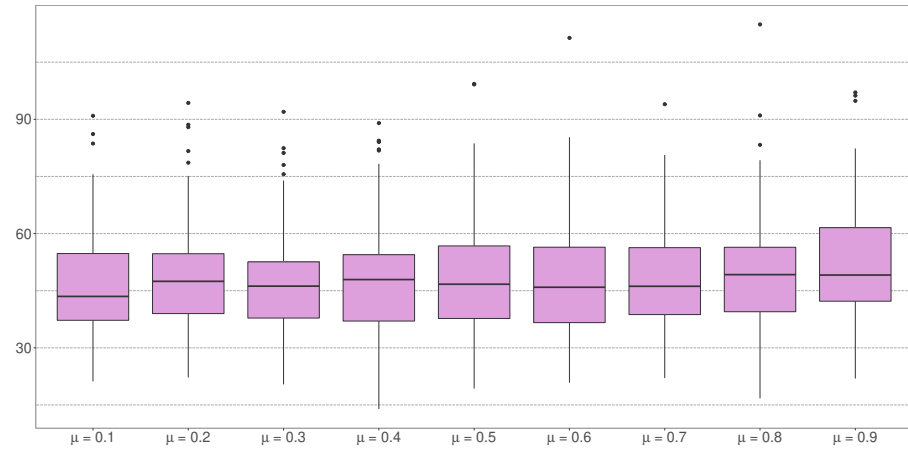

(b) Data with  $\sigma = 20$ .

Figure 1: Boxplots of the MSEs for the various model configurations tested when  $\mu$  is a hyperparameter, according to the data dispersion degree.

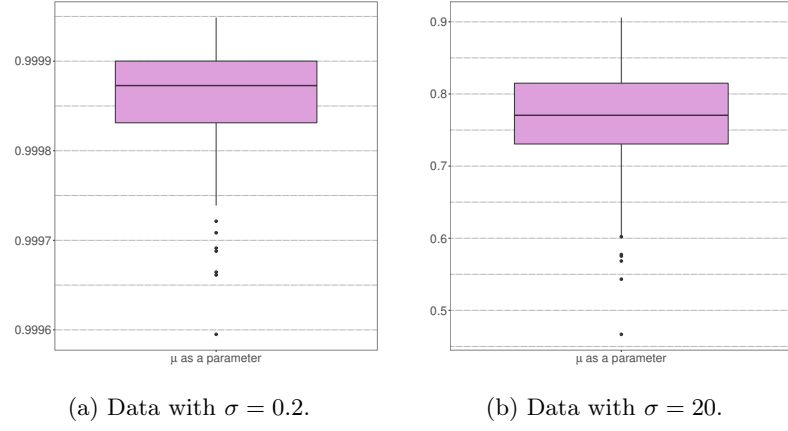

Figure 2: Boxplots of the metric (6) (presented in the article) for the model configuration with  $\mu$  as a parameter, according to the data dispersion degree.

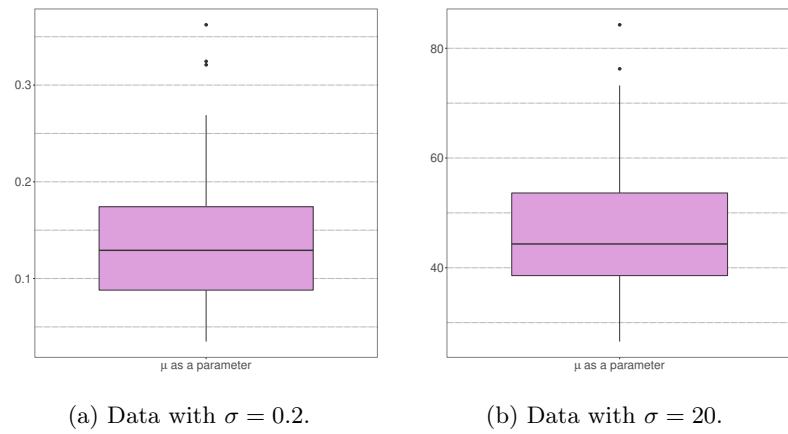

Figure 3: Boxplots of the MSEs for the model configuration with  $\mu$  as a parameter, according to the data dispersion degree.

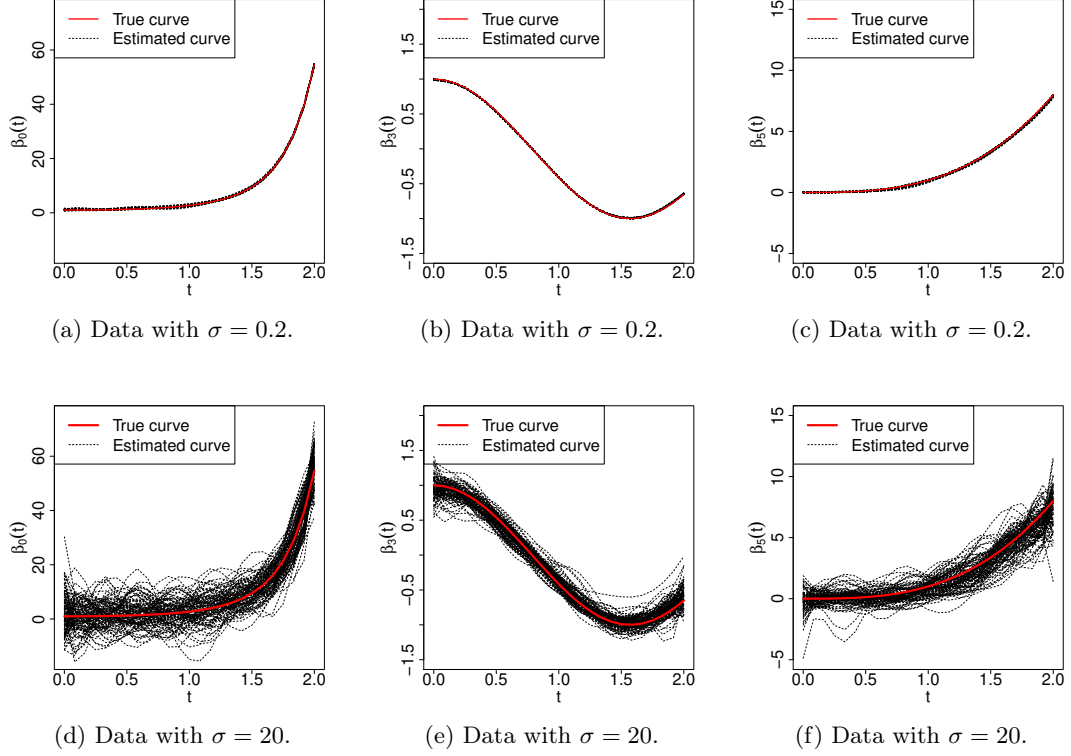

Figure 4: Intercept and partial functional coefficients (3<sup>rd</sup> and 5<sup>th</sup>, true in red and estimated for the replications in which the coefficients were selected in black) from the model that considers  $\mu$  as a parameter, according to the data dispersion degree (top row  $\sigma = 0.2$ , bottom row  $\sigma = 20$ ).

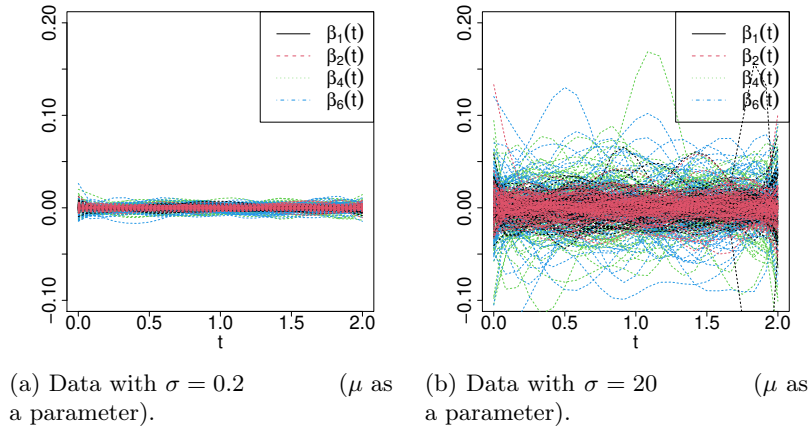

Figure 5: Estimated partial functional coefficients (1<sup>st</sup>, 2<sup>nd</sup>, 4<sup>th</sup> and 6<sup>th</sup>), from the model that considers  $\mu$  as a parameter, according to the data dispersion degree (for the replications whose coefficients were excluded among the total of 100 replications).

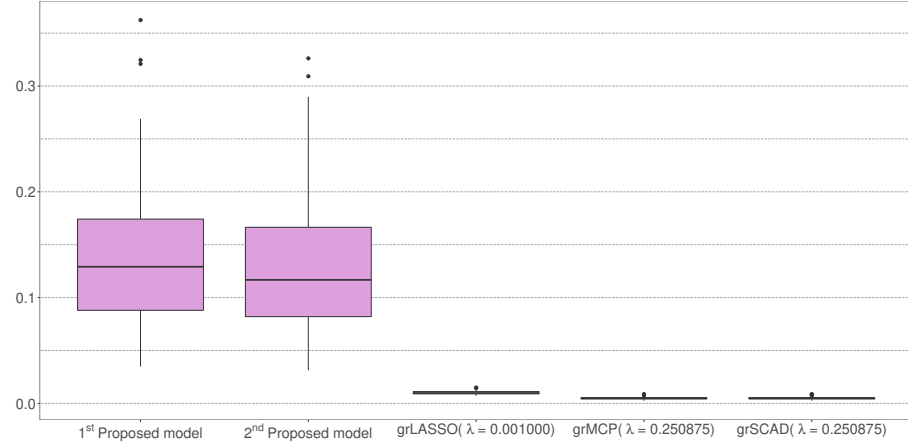

(a) Data with  $\sigma = 0.2$ .

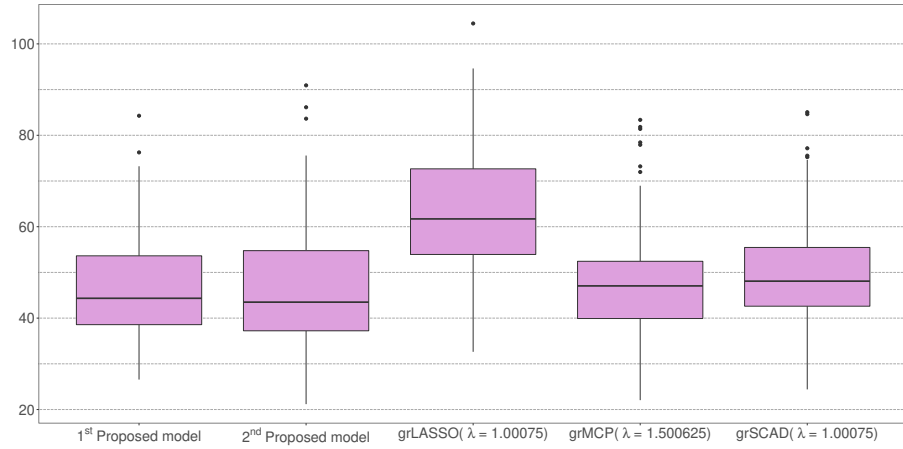

(b) Data with  $\sigma = 20$ .

Figure 6: Boxplots of the MSEs, according to the model used and the data dispersion degree. The “1<sup>st</sup> Proposed Model” is considered to be the version with  $\lambda = \sqrt{2}$  and  $\mu$  as a parameter, while the “2<sup>nd</sup> Proposed Model” is the version with  $\lambda = \sqrt{2}$  and  $\mu$  as a hyperparameter ( $\mu = 0.3$  para  $\sigma = 0.2$  e  $\mu = 0.1$  para  $\sigma = 20$ ).

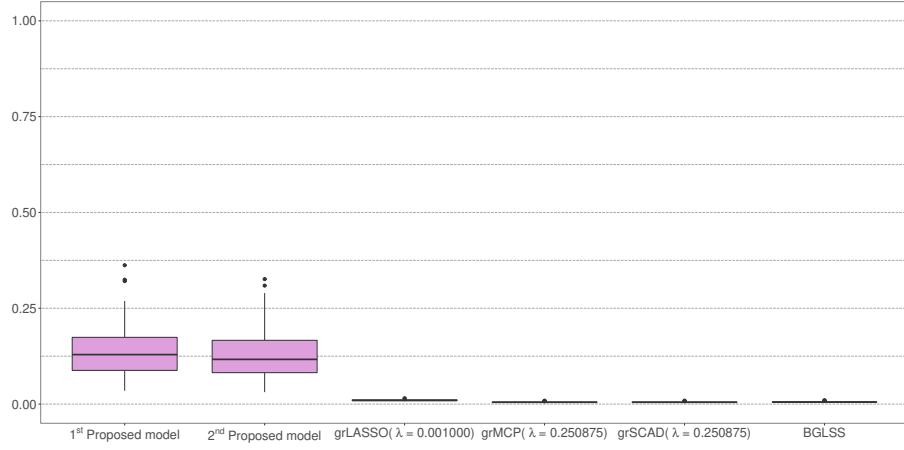

(a) Data with  $\sigma = 0.2$ .

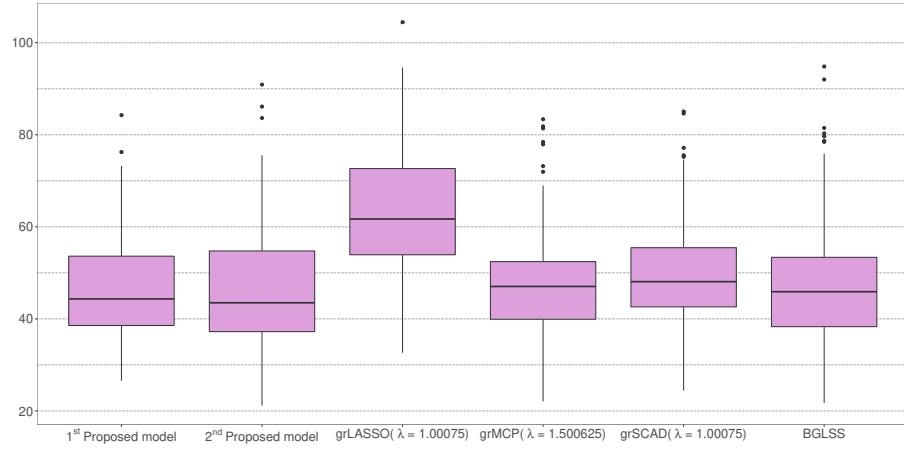

(b) Data with  $\sigma = 20$ .

Figure 7: Boxplots of the MSEs, according to the model used and the data dispersion degree. The “1<sup>st</sup> Proposed Model” is considered to be the version with  $\lambda = \sqrt{2}$  and  $\mu$  as a parameter, while the “2<sup>nd</sup> Proposed Model” is the version with  $\lambda = \sqrt{2}$  and  $\mu$  as a hyperparameter ( $\mu = 0.3$  para  $\sigma = 0.2$  e  $\mu = 0.1$  para  $\sigma = 20$ ).

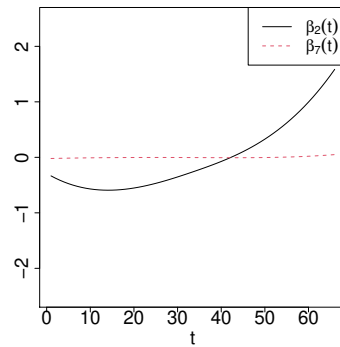

Figure 8: Estimated curves of the partial functional coefficients associated with the covariates that were excluded by the proposed model with  $K = 5$  ( $\beta_2(\cdot)$  for the HDI and  $\beta_7(\cdot)$  for the number of hospital beds per 10000 inhabitants).
